# Supplementary material for: Positive Focusing is Directly Useful
Source: arXiv:2411.09489 source file (2024-12-07)
Supplement: Supplementary file 1 [file toappendix.tex]

\gettoappendix {prop:local-postponement-gc}
\gettoappendix {prop:gc-postponement-vsc}
\gettoappendix {prop:local-termination-lsvsc}
\gettoappendix {thm:lppos-diamond}
\gettoappendix {prop:local-postponement-gc-xpos}
\gettoappendix {prop:vsc-gc-postponement}
\gettoappendix {prop:local-termination-positive}
\gettoappendix {l:good-bad}
\gettoappendix {l:good-ctx-properties}
\gettoappendix {prop:local-postponement-bad}
\gettoappendix {thm:postpone-bad}
\gettoappendix {thm:core-SN-equiv}
\gettoappendix {l:evar-absorption}
\gettoappendix {l:root-mult-simulation}
\gettoappendix {prop:sim-mult-steps}
\gettoappendix {l:egood-split}
\gettoappendix {prop:sim-us-exp-steps}
\gettoappendix {prop:charac-core-nfs}
\gettoappendix {prop:preserv-core-nfs}
\gettoappendix {thm:core-term-equiv}
